# Supplementary material for: Inferring entropy production from time-dependent moments
Source: arXiv:2310.16627 source file (2024-07-12)
Supplement: Supplementary file 1 [file supplementary.pdf]

# SUPPLEMENTARY INFORMATION: INFERRING ENTROPY PRODUCTION FROM TIME-DEPENDENT MOMENTS

Prashant Singh and Karel Proesmans
*Niels Bohr International Academy, Niels Bohr Institute, University of Copenhagen, Blegdamsvej 17, 2100 Copenhagen, Denmark*

## SUPPLEMENTARY NOTE 1: OPTIMIZING THE ENTROPY PRODUCTION RATE

Throughout our paper, we have considered a method that gives us the optimal value of mean total entropy produced $S_{\rm tot}(t_f)$ within fixed duration $[0, t_f]$ based on the information about moments. Here, we showcase another method that optimises the entropy production rate $\sigma(t) = \dot{S}_{\rm tot}(t)$ instead of the total dissipation $S_{\rm tot}(t)$. For simplicity, we focus on one dimensional case. The extension to higher dimension is quite straightforward. Moreover, we will refer to the method discussed in this section, where we minimise the rate $\sigma(t)$, as Method I and the method discussed in the main text, where we minimised the total dissipation $S_{\rm tot}(t)$ as Method II.
For systems obeying Langevin equation

$$\frac{dx}{dt} = (k_B T)^{-1} D \; F\left(x(t), t\right) + \zeta(t), \tag{S1}$$

the mean entropy production rate $\sigma(t)$ is given by [1]

$$\sigma(t) = \frac{k_B}{D} \int_{-\infty}^{\infty} dx \; P(x,t) \; v(x,t)^2. \tag{S2}$$

In order to optimize this with given moments

$$X_n(t) = \langle x^n(t) \rangle = \int_{-\infty}^{\infty} dx \; x^n P(x,t), \tag{S3}$$

$$\dot{X}_n(t) = \frac{d}{dt}\langle x^n(t) \rangle = n \int_{-\infty}^{\infty} dx \; x^{n-1} \; P(x,t) \; v(x,t), \tag{S4}$$

we consider the following objective function

$$\mathbb{L}(v) = \frac{D}{k_B}\sigma(t) + \sum_{i=1}^{m} \xi_i(t) \dot{X}_i(t), \tag{S5}$$

$$= \int_{-\infty}^{\infty} dx \; P(x,t) \left[ v(x,t)^2 + \sum_{i=1}^{m} i \; \xi_i(t) \; v(x,t) \right], \tag{S6}$$

where $\xi_i(t)$ for $1 \leq i \leq m$ are the Lagrange multipliers corresponding to the first $m$-moments. Now performing the minimisation $\left.\frac{\delta \; \mathbb{L}(v)}{\delta v(x,t)}\right|_{v^{12..m}(x,t)} = 0$, we obtain

$$v^{12..m}(x,t) = -\frac{1}{2} \sum_{i=1}^{m} \; i \; \xi_i(t) \; x^{i-1}, \tag{S7}$$

such that the Lagrange multipliers can be computed by inserting this solution in Eq. (S3). This gives a set of $m$ linear equations for $\xi_i(t), \; \xi_2(t), ..., \xi_m(t)$ as

$$-\frac{2}{i}\dot{X}_i(t) = \xi_1(t) X_{i-1}(t) + 2\xi_2(t) X_i(t) + ... + m\xi_m(t) X_{m-2+i}(t), \quad (\text{for } 1 \leq i \leq m). \tag{S8}$$

Solving these equations completely specifies $v(x,t)$ and plugging this in Eq. (S1), we find the optimal entropy production rate

$$\sigma(t) \geq \; \sigma^{12..m}(t) = \frac{k_B}{4D} \sum_{i,j=1}^{m} \xi_i(t) \; \xi_j(t) \; X_{i+j-2}(t). \tag{S9}$$

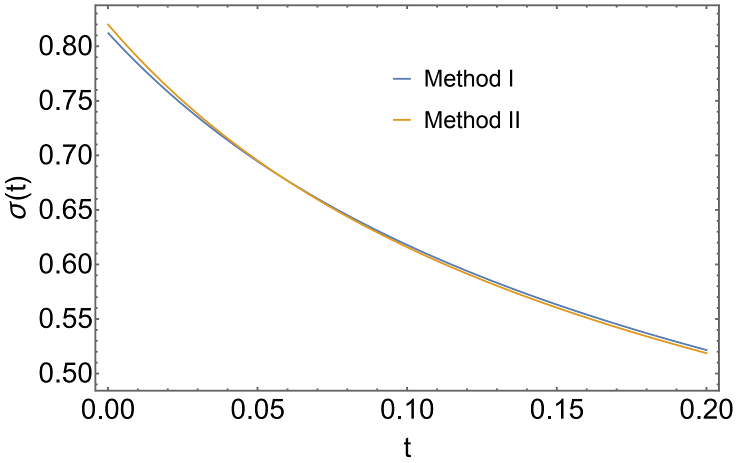


Supplementary figure 1. Comparison of two methods for free diffusion in Eq. (64) with given first four moments. Method I minimises the rate $\sigma(t)$ in Eq. (S1) whereas Method II minimises the total dissipation $S_{\rm tot}(t)$ as done in the main text. The two results are clearly different. Chosen parameters are $k_B = 1$ and $D = 0.2$.

In this case also, we can get the closed form solutions for $m = 2$

$$v^{12}(x,t) = \lambda_1(t) + \lambda_2(t)x, \tag{S10}$$

$$\sigma^{12}(t) = \frac{k_B}{D}\left[\frac{\dot{A}_2(t)^2}{4A_2(t)} + \dot{X}_1(t)^2\right]. \tag{S11}$$

where $A_2(t) = X_2(t) - X_1(t)^2$ is the variance of $x(t)$ and $\lambda$-functions are given by

$$\begin{cases} \lambda_1(t) &= \frac{2X_2(t)\dot{X}_1(t) - X_1(t)\dot{X}_2(t)}{2(X_2(t)-X_1^2(t))}, \\ \lambda_2(t) &= \frac{\dot{X}_2(t) - 2X_1(t)\dot{X}_1(t)}{2(X_2(t)-X_1^2(t))}. \end{cases} \tag{S12}$$

Both these results match with Eqs. (21) and (23) in the main text based on our previous method (where we optimise the total dissipation and not the rate). This means that for $m = 2$, the optimal value of $S_{\rm tot}(t_f)$ corresponds to optimising the rate $\sigma(t)$ at every time instant $0 \le t \le t_f$.

In the remaining part of this section, we prove that this does not remain true for general $m$ and the two methods yield different results. To see this, let us construct $y(x,t)$ corresponding to $v(x,t)$ in Eq. (S6) by using Eq. (6)

$$\dot{y}(x,t) = -\frac{1}{2}\sum_{i=1}^{m} i\ \xi_i(t)\ y\,(x,t)^{i-1}. \tag{S13}$$

Taking a time derivative, we find

$$\ddot{y}(x,t) = -\frac{1}{2}\sum_{i=1}^{m} i\ \dot{\xi}_i(t)\ y\,(x,t)^{i-1} + \frac{1}{4}\sum_{i,j=1}^{m} ij(i-1)\ \xi_i(t)\ \xi_j(t)\ y(x,t)^{i+j-3}. \tag{S14}$$

For general $m$, this does not match with Eq. (30) in the main text. For example, we get terms like $y(x,t)^m,\ y(x,t)^{m+1}$ and so on in Eq. (S13) which do not appear in Eq. (30). Therefore, two methods are inequivalent for general $m > 2$. This in-equivalence has also been illustrated in supplementary figure (1) for the free diffusion model considered in Eq. (64) by fixing the first four moments in Eqs.(67)-(69). In general, the method discussed in the main part of the paper will give a tighter bound for the total dissipation.

## SUPPLEMENTARY NOTE 2: BOUND $S^{12}_{\rm tot}(t_f)$ CONVERGES TO EXACT $S_{\rm tot}(t_f)$ FOR GAUSSIAN DISTRIBUTIONS

In this section, we prove that the bound $S^{12}_{\rm tot}(t_f)$ obtained in Eq. (21) of the main text converges with the exact average dissipation for Gaussian distributions. Let us begin with a general process $x(t)$ with time-dependent potential

$V(x,t) = \frac{K(t)}{2}x^2 - x\mathcal{F}(t)$ where $K(t)$ and $\mathcal{F}(t)$ are some arbitrary functions of time. This process satisfies the Langevin equation

$$\frac{dx}{dt} = -K(t)x + \mathcal{F}(t) + \sqrt{2D}\ \eta(t). \tag{S15}$$

If the initial position is drawn from the Gaussian distribution, then the process $x(t)$ also admits a Gaussian distribution given by

$$P(x,t) = \frac{1}{\sqrt{2\pi A_2(t)}} \exp\left[-\frac{(x - X_1(t))^2}{2A_2(t)}\right]. \tag{S16}$$

Combining this with Eq. (3), we can write the probability flux as

$$v(x,t) = \left(\frac{D}{A_2(t)} - K(t)\right)x + \left(\mathcal{F}(t) - \frac{DX_1(t)}{A_2(t)}\right). \tag{S17}$$

Since our aim is to express $v(x,t)$ completely in terms of moments and their time derivatives, we proceed to find both $K(t)$ and $\mathcal{F}(t)$ in terms of moments. Using Eq. (S16), it is easy to show that the variance $A_2(t)$ turns out to be

$$\frac{A_2(t)}{\mathcal{Z}^2(t)} = A_2(0) + 2D\int_0^t \frac{dw}{\mathcal{Z}(w)^2}, \qquad \text{with } \mathcal{Z}(t) = e^{-\int_0^t K(w)\ dw}. \tag{S18}$$

Taking time derivative on both sides, we get

$$K(t) - \frac{D}{A_2(t)} = \frac{\dot{A}_2(t)}{2A_2(t)}. \tag{S19}$$

This expresses the first term in Eq. (S16) in terms of the variance. Next we look at the second term. For this, we first express the mean as

$$\frac{X_1(t)}{\mathcal{Z}(t)} = X_1(0) + \int_0^t dw\ \frac{\mathcal{F}(w)}{\mathcal{Z}(w)}, \tag{S20}$$

and then take its time derivative to yield

$$\mathcal{F}(t) - \frac{DX_1(t)}{A_2(t)} = \dot{X}_1(t) + \frac{\dot{A}_2(t)\ X_1(t)}{2A_2(t)}. \tag{S21}$$

Substituting Eqs. (S18) and (S20) in Eq. (S16), we obtain

$$v(x,t) = -\frac{\dot{A}_2(t)}{2A_2(t)}\ x + \dot{X}_1(t) + \frac{\dot{A}_2(t)\ X_1(t)}{2A_2(t)}. \tag{S22}$$

Now the expression of flux involves only first two cumulants and their time derivatives. Finally, we use Eq. (4) to get the mean total entropy produced as

$$S_{\text{tot}}(t_f) = \frac{k_B}{D}\int_0^{t_f}\left[\dot{X}_1(t)^2 + \frac{\dot{A}_2(t)^2}{4A_2(t)}\right]. \tag{S23}$$

But this is also the bound $S^{12}_{\text{tot}}(t_f)$ derived in Eq. (21). Hence, we conclude that $S^{12}_{\text{tot}}(t_f)$ converges to its exact counterpart $S_{\text{tot}}(t_f)$ for Gaussian distributions. We remark that although the bound is saturated for Gaussian processes, there may still be other examples of non-Gaussian processes where the bound is also saturated as long as the probability flux in given by Eq. (23).

## SUPPLEMENTARY NOTE 3: SOLUTION OF EULER-LAGRANGE EQUATION IN GENERAL $d$ DIMENSION

This section presents a derivation of the Euler-Lagrange equation (41) in $d$ dimensions. For this, we first consider $\mathbf{y}(\mathbf{x},t)$ in Eq. (40) which is mathematically equivalent to switching from Eulerian description to the Lagrangian

description in fluid mechanics [2]. Using the equivalence of two descriptions, we have

$$\int_{-\infty}^{\infty} d\mathbf{x}\; P\left(\mathbf{x},t\right)\; g\left(\mathbf{x},t\right) = \int_{-\infty}^{\infty} d\mathbf{x}\; P_0\left(\mathbf{x}\right)\; g\left(\mathbf{y}(\mathbf{x},t),t\right), \tag{S24}$$

$$\int_{-\infty}^{\infty} d\mathbf{x}\; P\left(\mathbf{x},t\right)\; \mathbf{v}(\mathbf{x},t)\; g\left(\mathbf{x},t\right) = \int_{-\infty}^{\infty} d\mathbf{x}\; P_0\left(\mathbf{x}\right)\; \dot{\mathbf{y}}(\mathbf{x},t)\; g\left(\mathbf{y}(\mathbf{x},t),t\right). \tag{S25}$$

Plugging $g\left(\mathbf{x},t\right) = \delta\left(\mathbf{x} - \mathbf{y}(\mathbf{x}',t)\right)$, we get

$$P\left(\mathbf{y}(\mathbf{x}',t),t\right) = \frac{P_0(\mathbf{x}')}{\det\left(\nabla\mathbf{y}(\mathbf{x}',t)\right)}. \tag{S26}$$

On the other hand, putting $g\left(\mathbf{x},t\right) = \mathbf{v}(\mathbf{x},t)^2$ in Eq. (S23), we obtain

$$S_{\rm tot}(t_f) = \frac{k_B}{D}\int_0^{t_f} dt\; \int_{-\infty}^{\infty} d\mathbf{x}\; P_0(\mathbf{x})\; \dot{\mathbf{y}}\left(\mathbf{x},t\right)^2. \tag{S27}$$

In fact, one can use $\mathbf{y}\left(\mathbf{x},t\right)$ to recast the optimisation of action $\mathbb{S}\left(\mathbf{x},\dot{\mathbf{v}},t_f\right)$ in Eq. (39) as an optimisation problem in $\mathbf{y}\left(\mathbf{x},t\right)$. To see this, we first rewrite $\mathbb{S}\left(\mathbf{x},\dot{\mathbf{v}},t_f\right)$ as

$$\begin{aligned}\mathbb{S}\left(\mathbf{y},\dot{\mathbf{y}},t_f\right) = &\int_0^{t_f} dt \int_{-\infty}^{\infty} d\mathbf{x}\; P_0\left(\mathbf{x}\right)\left[\dot{\mathbf{y}}\left(\mathbf{x},t\right)^2 + \sum_{i=1}^{d}\mu_i(t)\; y_i\left(\mathbf{x},t\right) + \sum_{i,j=1}^{d}\lambda_{ij}(t)\; y_i\left(\mathbf{x},t\right) y_j\left(\mathbf{x},t\right)\right]\\ &+\int_{-\infty}^{\infty} d\mathbf{x}\; P_0\left(\mathbf{x}\right)\left[\sum_{i=1}^{d}\alpha_i(t_f)\; y_i\left(\mathbf{x},t_f\right) + \sum_{i,j=1}^{d}\beta_{ij}(t_f)\; y_i\left(\mathbf{x},t_f\right) y_j\left(\mathbf{x},t_f\right)\right].\end{aligned} \tag{S28}$$

For a small change in path $\mathbf{y}\left(\mathbf{x},t\right) \to \mathbf{y}\left(\mathbf{x},t\right) + \delta\mathbf{y}\left(\mathbf{x},t\right)$, the total change in action is given by

$$\begin{aligned}\delta\mathbb{S} = &\int_0^{t_f} dt \int_{-\infty}^{\infty} d\mathbf{x}\; P_0\left(\mathbf{x}\right)\sum_{i=1}^{d}\left[-2\ddot{y}_i(\mathbf{x},t) + \mu_i(t) + \sum_{j=1}^{d}\tilde{\lambda}_{ij}(t)\; y_j(\mathbf{x},t)\right]\delta y_i(\mathbf{x},t)\\ &+\int_{-\infty}^{\infty} d\mathbf{x}\; P_0\left(\mathbf{x}\right)\; \sum_{i=1}^{d}\left[2\dot{y}_i\left(\mathbf{x},t_f\right) + \alpha_i(t_f) + \sum_{j=1}^{d}\tilde{\beta}_{ij}(t_f)\; y_j\left(\mathbf{x},t_f\right)\right]\delta y_i(\mathbf{x},t_f)\\ &-2\int_{-\infty}^{\infty} d\mathbf{x}\; P_0\left(\mathbf{x}\right)\; \sum_{i=1}^{d}\dot{y}_i\left(\mathbf{x},0\right)\delta y_i(\mathbf{x},0).\end{aligned} \tag{S29}$$

where $\tilde{\lambda}_{ij}(t) = \lambda_{ij}(t) + \lambda_{ji}(t)$ and $\tilde{\beta}_{ij}(t) = \beta_{ij}(t) + \beta_{ji}(t)$. For optimal path, this change in action should vanish. Vanishing of the first line for arbitrary $\delta y_i\left(\mathbf{x},t\right)$ gives the Euler-Lagrange equation

$$2\ddot{y}_i(\mathbf{x},t) = \mu_i(t) + \sum_{j=1}^{d}\tilde{\lambda}_{ij}(t)\; y_j(\mathbf{x},t). \tag{S30}$$

On the other hand, we get appropriate boundary conditions by demanding vanishing of the other two lines. Since, we begin with fixed initial condition $\mathbf{y}(\mathbf{x},0) = \mathbf{x}$, the third line in Eq. (S28) trivially goes to zero. However, the value of $\mathbf{y}(\mathbf{x},t_f)$ at the final time is not fixed which means $\delta\mathbf{y}\left(\mathbf{x},t_f\right) \neq 0$. Hence for the change $\delta\mathbb{S}$ to become zero, we must have the pre-factor associated with $\delta y_i\left(\mathbf{x},t_f\right)$ in the second line equal to zero. Thus, we derive the following boundary conditions in time

$$2\dot{y}_i\left(\mathbf{x},t_f\right) + \alpha_i(t_f) + \sum_{j=1}^{d}\tilde{\beta}_{ij}(t_f)\; y_j\left(\mathbf{x},t_f\right) = 0, \tag{S31}$$

$$y_i(\mathbf{x},0) = x_i. \tag{S32}$$

Due to the linearity of Eq. (S29) in $\mathbf{y}(\mathbf{x},t)$, the general solution satisfies

$$\dot{y}_i\left(\mathbf{x},t\right) = -\frac{\nu_i(t)}{2} - \sum_{j=1}^{d}\frac{\gamma_{ij}(t)}{2}\; y_j\left(\mathbf{x},t\right), \qquad \text{for } 0 \le t \le t_f. \tag{S33}$$

In order to see that this is consistent with Eq. (S29), we take its time derivative and compare the resulting $\ddot{y}_i(\mathbf{x}, t)$ with Eq. (S29). This gives rise to the following relations

$$\mu_i(t) = -\dot{\nu}_i(t) + \frac{1}{2}\sum_{l=1}^{d} \frac{\gamma_{il}(t)\ \nu_l(t)}{2}, \quad \text{and} \quad \tilde{\lambda}_{ij}(t) = -\dot{\gamma}_{ij}(t) + \sum_{l=1}^{d} \frac{\gamma_{il}(t)\ \gamma_{lj}(t)}{2}. \tag{S34}$$

These relations ensure that Eqs. (S29) and (S32) are consistent with each other. To summarize, we have derived the solution for the optimal path. We now have to simply insert this solution in Eq. (S26) to get the bound on total dissipation. However, before that we need to specify $\nu(t)$ and $\gamma(t)$ functions. For this, we use the definition of moments

$$X_1^i(t) = \int_{-\infty}^{\infty} d\mathbf{x}\ P_0(\mathbf{x})\, y_i(\mathbf{x}, t), \quad \text{and } X_2^{i,j}(t) = \int_{-\infty}^{\infty} d\mathbf{x}\ P_0(\mathbf{x})\, y_i(\mathbf{x}, t)\, y_j(\mathbf{x}, t). \tag{S35}$$

and take their time derivative to yield

$$\nu_i(t) = -2\dot{X}_1^i(t) - \sum_{l=1}^{d} \gamma_{il}(t)\ X_1^l(t), \tag{S36}$$

$$-2\dot{A}_{ij}(t) = \sum_{l=1}^{d} \left[\gamma_{il}(t) A_{jl}(t) + \gamma_{jl}(t) A_{il}(t)\right], \tag{S37}$$

where $A_{ij}(t) = X_2^{i,j}(t) - X_1^i(t) X_1^j(t)$. We have quoted this result in Eq. (42) of the main text.

### A. Simplification in two dimensions

For two dimensional case, we can explicitly solve Eqs. (S36) and obtain

$$\gamma_{11}(t) = \frac{-A_{22}(t)\dot{A}_{11}(t)\left[A_{11}(t) + A_{22}(t)\right] + 2A_{12}(t)A_{22}(t)\dot{A}_{12}(t) + A_{12}(t)^2\left[\dot{A}_{11}(t) - \dot{A}_{22}(t)\right]}{\left[A_{11}(t) + A_{22}(t)\right]\left[A_{11}(t)A_{22}(t) - A_{12}(t)^2\right]},$$

$$\gamma_{22}(t) = \frac{-A_{11}(t)\dot{A}_{22}(t)\left[A_{11}(t) + A_{22}(t)\right] + 2A_{12}(t)A_{11}(t)\dot{A}_{12}(t) + A_{12}(t)^2\left[-\dot{A}_{11}(t) + \dot{A}_{22}(t)\right]}{\left[A_{11}(t) + A_{22}(t)\right]\left[A_{11}(t)A_{22}(t) - A_{12}(t)^2\right]},$$

$$\gamma_{12}(t) = \frac{\dot{A}_{11}(t)A_{12}(t)A_{22}(t) + A_{11}(t)A_{12}(t)\dot{A}_{22}(t) - 2A_{11}(t)\dot{A}_{12}(t)A_{22}(t)}{\left[A_{11}(t) + A_{22}(t)\right]\left[A_{11}(t)A_{22}(t) - A_{12}(t)^2\right]}.$$

Plugging them in formula

$$S_{\text{tot}}(t_f) = \frac{k_B}{D}\int_0^{t_f} dt \int_{-\infty}^{\infty} d\mathbf{x}\ P_0(\mathbf{x})\ \dot{\mathbf{y}}(\mathbf{x}, t)^2, \tag{S38}$$

we obtain the total dissipation bound as

$$S_{\text{tot}}^{12}(t_f) = \frac{k_B}{D}\int_0^{t_f} dt \left[\dot{X}_1^1(t)^2 + \frac{\dot{A}_{11}(t)^2}{4A_{11}(t)} + \dot{X}_1^2(t)^2 + \frac{\dot{A}_{22}(t)^2}{4A_{22}(t)} + \frac{\left\{A_{12}(t)\frac{d}{dt}\left(A_{11}(t)A_{22}(t)\right) - 2A_{11}(t)A_{22}(t)\dot{A}_{12}(t)\right\}^2}{4A_{11}(t)A_{22}(t)\left\{A_{11}(t) + A_{22}(t)\right\}\left\{A_{11}(t)A_{22}(t) - A_{12}(t)^2\right\}}\right]. \tag{S39}$$

This result has been written in Eq. (48) in the main text.

## SUPPLEMENTARY NOTE 4: EFFECT OF TRAJECTORY NUMBER ON THE LOWER BOUND

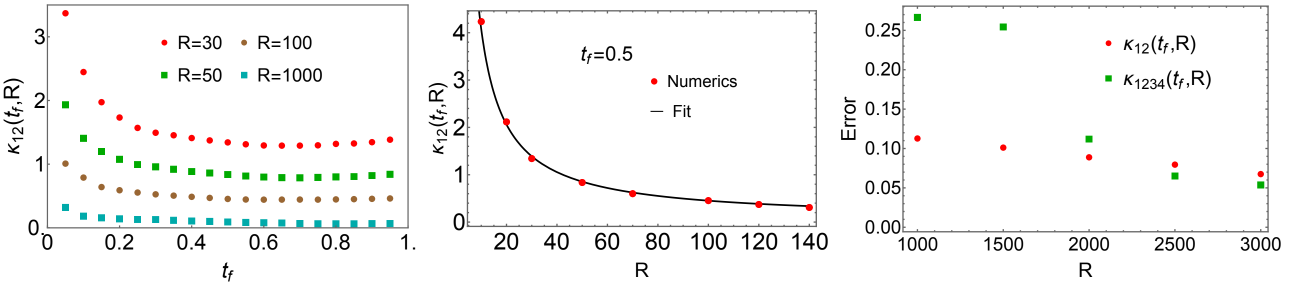


Supplementary figure 2. Left panel shows the plot of $\kappa_{12}(t_f, R)$ as a function of $t_f$ for different values of $R$ (the number of trajectories). With increasing $R$, we see decrease in the value of $\kappa_{12}(t_f, R)$. This is further illustrated on the middle panel where we plot $\kappa_{12}(t_f, R)$ vs $R$ for a fixed $t_f = 0.5$. In this panel, the numerical data (shown in red) is fitted by $\kappa_{12}(t_f, R) = a_0 + b_0/R$ (shown in black) with $a_0 = 0.05,\ b_0 = 40.198$. In the rightmost panel, we have shown a comparison between $\kappa_{12}(t_f, R)$ and $\kappa_{1234}(t_f, R)$ for a fixed $t_f = 0.5$.

In the main text, we presented a theoretical example where we obtained the lower bound either analytically or numerically. This was possible using the expressions of the moments. However, while calculating moments from the available trajectories, one still has to deal with the noise, and its effect becomes more pronounced if the number of trajectories (denoted by $R$) is small. This, in turn, affects the accuracy of the lower bound. Below, we quantitatively demonstrate this effect of the finite trajectory on the lower bound.

To this aim, we generate $R$ trajectories following the Langevin equation (64), and use them to obtain the moments $X_1(t),\ X_2(t), ..., X_m(t)$. Employing our method, we then calculate the lower bound $S_{\text{tot}}^{12..m}(t_f)\big|_{R1}$. Recall that while for first two moments, we have an analytic formula for the lower bound in Eq. (70), for higher moment, we obtain it numerically. We next generate another set of $R$ trajectories and calculate $S_{\text{tot}}^{12..m}(t_f)\big|_{R2}$. Proceeding this way $\mathcal{N}$ times with ($\mathcal{N} \gg 1$), we obtain estimates $S_{\text{tot}}^{12..m}(t_f)\big|_{R3}$, $S_{\text{tot}}^{12..m}(t_f)\big|_{R4}$, ....$S_{\text{tot}}^{12..m}(t_f)\big|_{R\mathcal{N}}$. Ideally all these values should coincide with our lower bound $S_{\text{tot}}^{12..m}(t_f)$. However, for small $R$, each of these estimates will be different. To study this fluctuation, we look at the following quantity:

$$\kappa_{12..m}(t_f, R)^2 = \frac{1}{\mathcal{N}} \sum_{j=1}^{\mathcal{N}} \left( \frac{S_{\text{tot}}(t_f) - S_{\text{tot}}^{12..m}(t_f)\big|_{Rj}}{S_{\text{tot}}(t_f)} \right)^2, \quad \text{with } \mathcal{N} \gg 1. \tag{S40}$$

Here $S_{\text{tot}}(t_f)$ denotes the exact mean entropy production whose expression is given in Eq. (66). For $R \to \infty$, this quantity converges with the true error between the lower bound and the exact value of the entropy production. However, for finite $R$, $\kappa_{12..m}(t_f, R)$ also includes the error due to the noise in the system. We first focus on the $m = 2$ case. In supplementary figure 2 (left panel), we have plotted this quantity as a function of $t_f$ for four different values of $R$. For small values such as $R = 30$, we see that $\kappa_{12}(t_f, R)$ is quite large indicating that the effect of noise is quite prominent. Here our estimate of the lower bound is less accurate. On the other hand, for larger values of $R$, error $\kappa_{12}(t_f, R)$ decreases and the accuracy of our bound increases. This is further illustrated on the middle panel where we plot $\kappa_{12}(t_f, R)$ vs $R$ for a fixed $t_f = 0.5$. Here, we observe that $\kappa_{12}(t_f, R)$ decays as $(a_0 + b_0/R)$ with the trajectory number. Remember that for $R \to \infty$, the effect of noise is no longer present and then $\kappa_{12}(t_f, R)$ should converge with the error in Eq. (74).

We next consider $m = 4$ where our method becomes numerical. For a small number of trajectories, the noise has a greater impact on higher moments compared to lower moments. Here, we expect the estimate $S_{\text{tot}}^{1234}(t_f)$ to deviate significantly from its true value compared to the estimate $S_{\text{tot}}^{12}(t_f)$ with lower moments. On the other hand, when $R$ is significantly large, the accuracy of $S_{\text{tot}}^{1234}(t_f)$ always surpasses that of $S_{\text{tot}}^{12}(t_f)$. To demonstrate this, we have plotted $\kappa_{1234}(t_f, R)$ and $\kappa_{12}(t_f, R)$ in the right panel of supplementary figure 2. While for larger values of $R$, $\kappa_{12}(t_f, R)$ exceeds $\kappa_{1234}(t_f, R)$, the opposite is seen when $R$ is not large. However, performing this comparison for small $R$ turns out to be challenging and our numerical code quickly becomes unstable for $S_{\text{tot}}^{1234}(t_f)\big|_{Rj}$. A further investigation is required to understand the role of trajectory number on our lower bound with higher moments.

## SUPPLEMENTARY NOTE 5: MEASUREMENT NOISE

In this section, we will investigate the effect due to the measurement noise in our bound. While acquiring the trajectory data, there are intrinsic errors that occur due to the data measurement. Due to this, the observed data is

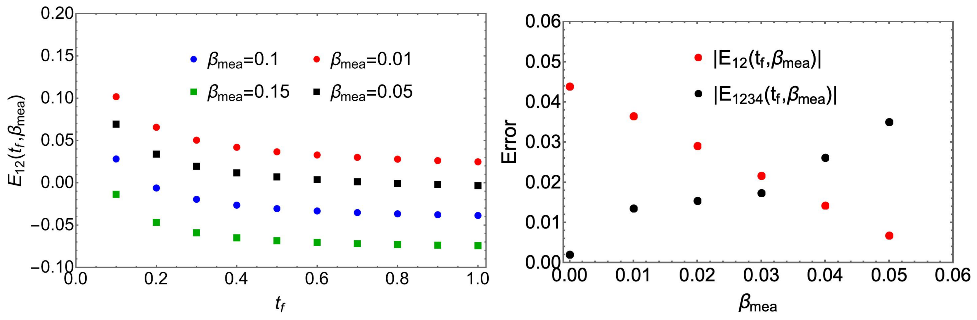


Supplementary figure 3. This figure shows the impact of measurement noise on the lower bound. In left panel, we have plotted the error $E_{12}\left(t_f, \beta_{\text{mea}}\right)$ as a function of $t_f$ for different values of $\beta_{\text{mea}}$. In the right panel, we have compared the absolute values of $E_{12}\left(t_f, \beta_{\text{mea}}\right)$ and $E_{1234}\left(t_f, \beta_{\text{mea}}\right)$ by varying $\beta_{\text{mea}}$ but keeping the final time fixed to $t_f = 0.5$.

different than the actual value [3]. This, in turn, affects the moments and hence the lower bound. We illustrate this for the free diffusion model.

Let us consider that the trajectory of total time $t$ is obtained with a resolution $\Delta t$ such that $N\Delta t = t$. At time-step $j$, the actual particle position is $x_j^{\text{act}}$, while the measured position is $x_j^{\text{mea}}$. We include the measurement noise as follows [3]:

$$x_j^{\text{mea}} = x_j^{\text{act}} + l_j, \tag{S41}$$

where $l_j$ is a Gaussian white noise with zero mean and variance $\langle l_i l_j \rangle = \delta_{i,j}\sigma_{\text{mea}}^2$. Note that $x_j^{\text{act}}$ follows the dynamics in Eq. (64)

$$x_j^{\text{act}} = x_{j-1}^{\text{act}} + \sqrt{2D\Delta t}\ \eta_j. \tag{S42}$$

Plugging this in Eq. (S41)

$$x_j^{\text{mea}} = x_{j-1}^{\text{act}} + \sqrt{2D\Delta t}\ \eta_j + l_j, \tag{S43}$$

$$= x_{j-1}^{\text{mea}} + \sqrt{2D\Delta t}\ \eta_j + l_j - l_{j-1}. \tag{S44}$$

Since, at time-step $j = 0$, the distribution of $x_0$ is assumed to be given, we take $l_0 = 0$ and $x_0^{\text{mea}} = 0$. With this, Eq. (S43) can now be iteratively solved. The second and the fourth moment turns out to be

$$X_2^{\text{mea}}(t) = \frac{\Gamma\left(\frac{3}{4}\right)}{\Gamma\left(\frac{1}{4}\right)} + (2D + \beta_{\text{mea}})t, \tag{S45}$$

$$X_4^{\text{mea}}(t) = \frac{1}{4} + \frac{6\Gamma\left(\frac{3}{4}\right)}{\Gamma\left(\frac{1}{4}\right)}(2D + \beta_{\text{mea}})t + 3(2D + \beta_{\text{mea}})^2 t^2, \tag{S46}$$

where $\beta_{\text{mea}} = \sigma_{\text{mea}}^2/\Delta t$, and it quantitatively captures the effect of the measurement noise. Using Eqs. (S44) and (S45), we can now obtain the lower bounds. For example, the bound due to the first two moments is

$$S_{\text{tot}}^{12}(t_f)\big|_{\text{mea}} = \frac{k_B}{2}\left(1 + \frac{\beta_{\text{mea}}}{2D}\right)\ \log\left(\frac{(2D + \beta_{\text{mea}})t_f + \frac{\Gamma\left(\frac{3}{4}\right)}{\Gamma\left(\frac{1}{4}\right)}}{\frac{\Gamma\left(\frac{3}{4}\right)}{\Gamma\left(\frac{1}{4}\right)}}\right). \tag{S47}$$

In absence of the measurement noise, $\beta_{\text{mea}} = 0$ and this result matches with the expression in Eq. (70). We next use this result to obtain the measurement error as

$$E_{12}\left(t_f, \beta_{\text{mea}}\right) = \frac{S_{\text{tot}}(t_f) - S_{\text{tot}}^{12}(t_f)\big|_{\text{mea}}}{S_{\text{tot}}(t_f)}. \tag{S48}$$

In supplementary figure 3 (left panel), we have plotted this error as a function of the observation time $t_f$ for different values of $\beta_{\text{mea}}$. For $\beta_{\text{mea}} = 0$, the error is always positive. As $\beta_{\text{mea}}$ increases from zero to a small value, we observe that

$E_{12}(t_f, \beta_{\rm mea})$ approaches zero, implying that the bound becomes more accurate. However, with a further increase in $\beta_{\rm mea}$, the error becomes negative, causing the bound to overestimate the entropy production.

Next, we examine the impact of $\beta_{\rm mea}$ on $S_{\rm tot}^{1234}(t_f)$. Using the moments in Eqs. (S44) and (S45), we follow the recipe outlined in the paper and calculate the error $E_{1234}(t_f, \beta_{\rm mea})$ similar to Eq. (S47). The right panel of supplementary figure 3 depicts a comparison of $E_{12}(t_f, \beta_{\rm mea})$ and $E_{1234}(t_f, \beta_{\rm mea})$. As clear from this figure, while for lower values of $\beta_{\rm mea}$, the bound $S_{\rm tot}^{1234}(t_f)$ is more accurate compared to $S_{\rm tot}^{12}(t_f)$, for higher values of $\beta_{\rm mea}$, the effect of noise on higher moments is large and $S_{\rm tot}^{1234}(t_f)$ becomes less accurate.

## SUPPLEMENTARY NOTE 6: EXPERIMENTAL PROTOCOLS

| cycle time | m(t) | g(t) | f(t) | action |
|---|---|---|---|---|
| $t \in [0, 0.25t_f]$ | $\left(1 - \frac{t}{0.25t_f}\right)^2$ | 1 | 0 | symmetrize potential |
| $t \in [0.25t_f, 0.4t_f]$ | 0 | $\left(2 - \frac{t}{0.25t_f}\right)^2$ | 0 | lower barrier |
| $t \in [0.4t_f, 0.6t_f]$ | 0 | $\left(2 - \frac{t}{0.25t_f}\right)^2$ | $\left(\frac{t/t_f - 0.4}{0.2}\right)$ | tilt |
| $t \in [0.6t_f, 0.65t_f]$ | 0 | $\left(2 - \frac{t}{0.25t_f}\right)^2$ | 1 | raise barrier |
| $t \in [0.65t_f, 0.75t_f]$ | 0 | $\left(2 - \frac{t}{0.25t_f}\right)^2$ | $\left(1 - \frac{t/t_f - 0.65}{0.1}\right)$ | Untilt |
| $t \in [0.75t_f, t_f]$ | $\left(3 - \frac{t}{0.25t_f}\right)^2$ | 1 | 0 | asymmetrize potential |

Supplementary table I. Expressions of the dimensionless functions $m(t)$, $g(t)$ and $f(t)$ that are used in order to change the double-well potential in the bit erasure experiment.

| Cycle time | No. of trajectories |
|---|---|
| 13.36 | 40 |
| 14.89 | 53 |
| 17.30 | 40 |
| 19.79 | 28 |
| 21.19 | 20 |
| 28.59 | 22 |
| 40.78 | 16 |

Supplementary table II. Number of trajectories considered for different cycle times (rescaled) in the experiment.

## SUPPLEMENTARY NOTE 7: SPATIALLY-DEPENDENT DIFFUSION COEFFICIENT

In this section, we will discuss how our main results change in the presence of a spatially dependent diffusion coefficient. Throughout this section, we will focus on one-dimensional systems, but the results can easily be extended to higher-dimensional systems.

In particular, we will show that one can infer the entropy production numerically, provided that one has access to the spatial dependence of the diffusion coefficient, $D(x)$ and that one can access to $\langle D(x)x^i\rangle$. Firstly, we note that the Fokker-Planck equation (in the Stratonovich convention) is still given by Eq. (2), but that the probability flux now is given by

$$v(x,t) = \frac{D(x)F(x,t)}{k_B T} - \frac{1}{2}\nabla D(x) - D(x)\nabla \ln P(\mathbf{x},t). \tag{S49}$$

One can verify that full control over the force-field still implies full control over the probability flux.

The entropy production is now given by [4]

$$S_{\rm tot}(t_f) = k_B \int_0^{t_f} dt \int_{-\infty}^{\infty} dx\, \frac{P(x,t)\, v(x,t)^2}{D(x)}. \tag{S50}$$

Doing the same analysis as in the main text leads to an action

$$\mathbb{S}\left(y,\dot{y},t_f\right)=\int_0^{t_f}dt\int_{-\infty}^{\infty}dx\ P_0(x)\ \left[\frac{\dot{y}(x,t)^2}{D(y(x,t)}+\sum_{i=1}^{m}\mu_i(t)\ y(x,t)^i\right]+\int_{-\infty}^{\infty}dx\ P_0(x)\ \sum_{i=1}^{m}\zeta_i(t_f)\ y(x,t_f)^i.$$

that needs to be minimised under the constraints

$$2\dot{y}(x,t_f)=-D(y(x,t_f))\sum_{i=1}^{m}i\ \zeta_i(t_f)\ y(x,t_f)^{i-1},\qquad y(x,0)=x. \tag{S51}$$

Doing the same analysis as before leads to

$$2\ddot{y}(x,t)=\frac{\dot{y}(x,t)^2D'(y(x,t))}{D(y(x,t))}+D(y(x,t))\sum_{i=1}^{m}i\ \mu_i(t)\ y(x,t)^{i-1}, \tag{S52}$$

$$-\frac{2}{i}\dot{X}_i(t_f)=\zeta_1(t_f)\left\langle D(x)x^{i-1}\right\rangle(t_f)+2\zeta_2(t_f)\left\langle D(x)x^{i}\right\rangle(t_f)+...+m\zeta_m(t_f)\left\langle D(x)x^{m-2+i}\right\rangle(t_f), \tag{S53}$$

$$\ddot{X}_i(t)=\mathcal{B}_i(t)+\mathcal{E}_i(t)+\frac{i}{2}\left[\mu_1(t)\left\langle D(x)x^{i-1}\right\rangle(t)+2\mu_2(t)\left\langle D(x)x^{i}\right\rangle(t)+...+m\mu_m(t)\left\langle D(x)x^{m-2+i}\right\rangle(t)\right], \tag{S54}$$

where $\mathcal{B}_i(t)$ is given in Eq. (35) and $\mathcal{E}_i(t)$ is defined as

$$\mathcal{E}_i(t)=\frac{i}{2}\int_{-\infty}^{\infty}dx\ P_0(x)\ \frac{D'(y(x,t))}{D(y(x,t))}\ y(x,t)^{i-1}\ \dot{y}(x,t)^2. \tag{S55}$$

These equations can be solved numerically in exactly the same way as before, leading to a bound for systems with spatially dependent diffusion coefficients.


[1] L. Peliti and S. Pigolotti, *Stochastic Thermodynamics: An Introduction* (Princeton University Press, 2021).

[2] J.-D. Benamou and Y. Brenier, A computational fluid mechanics solution to the monge-kantorovich mass transfer problem, Numerische Mathematik **84**, 375 (2000).

[3] S. Thapa, M. A. Lomholt, J. Krog, A. G. Cherstvy, and R. Metzler, Bayesian analysis of single-particle tracking data using the nested-sampling algorithm: maximum-likelihood model selection applied to stochastic-diffusivity data, Physical Chemistry Chemical Physics **20**, 29018 (2018).

[4] R. E. Spinney and I. J. Ford, Entropy production in full phase space for continuous stochastic dynamics, Physical Review E **85**, 051113 (2012).
